# Supplementary material for: Meta-Learning to Cluster
Source: arXiv:1910.14134 source file (2019-10-30)
Supplement: Supplementary file 1 [file appendix.tex]

\appendix
\section{The Possibility of Meta-Clustering}
\label{app:possibility}
Kleinberg's impossibility theorem \citep{DBLP:conf/nips/Kleinberg02} suggests that clustering is impossible because there is no clustering algorithm that can satisfy the three very intuitive axioms that any clustering algorithm should follow. In this section, we will discuss how we can reframe the three axioms for meta-clustering to circumvent impossibility theorem. Considering a finite set of points $X$ and associated symmetric distance function $d \in D(X)$ where $D(X)$ contains all the possible distance functions for $X$. Clustering algorithm $\mathcal{A}$ takes in distance function $d$ and returns partitions of $X$. Following the formulation in \citet{DBLP:conf/nips/Garg18}, the three axioms can be described as follows.
\\

\noindent \textbf{Scale-Invariance}. For any distance function $d$ and any $\alpha > 0$, $\mathcal{A}(d) = \mathcal{A}(\alpha \cdot d)$.
    \\
    
\noindent \textbf{Richness.} For any finite $X$ and clustering $\mathcal{C}$ of $X$, there exists a distance function $d \in D(X)$ such that $\mathcal{A}(d) = \mathcal{C}$.
   \\
   
\noindent \textbf{Consistency.} Let $d, d' \in D(X)$ such that $\mathcal{A}(d) = \mathcal{C}$, and for all $x, x' \in X$, if $x, x'$ are in the same cluster in $\mathcal{C}$ then $d'(x,x') \leq d(x,x')$, while if $x,x'$ are in different clusters in $\mathcal{C}$ then $d'(x,x') \geq d(x,x')$. Then the axiom demands $\mathcal{A}(d') = \mathcal{A}(d)$.
\\

\citet{DBLP:conf/nips/Garg18} suggests a re-framing of the axioms for meta-clustering. Specifically, by introducing a variant of Scale-Invariance, \citet{DBLP:conf/nips/Garg18} proves that there is a meta-clustering algorithm that satisfies the new Scale-Invariance axiom and whose output always satisfies Richness and Consistency. Different from their version, we consider a different formulation of meta clustering algorithms and also gives variants of Richness and Consistency targeting meta clustering algorithms. 

Suppose $\mathcal{M}$ is a meta clustering algorithm as described in Section~\ref{sec:meta-setup}. We can consider $\mathcal{M}$ to consist of two steps. First, $\mathcal{M}$ takes distance function $d$ of dataset $X$ and outputs a clustering algorithm $\mathcal{A}$, i.e. $\mathcal{M}[d] = \mathcal{A}$. Second, the clustering algorithm $\mathcal{A}$, in turn, will do the clustering via $d$ and outputs a partition $\mathcal{C}$, i.e. $\mathcal{A}(d) = \mathcal{C}$. Essentially, $\mathcal{M}[d](d) = \mathcal{C}$. $\mathcal{M}$ is trained in the meta-training phase to adapt to clustering tasks, provided with datasets and true clustering labels, unlike \citet{DBLP:conf/nips/Garg18} which returns one clustering algorithm based on training datasets and labels. In our case, LSTM does both the steps, performing clustering on input data $X$ but also adapting to $X$. The adaptation happens through the change of activations and gates' values inside LSTM. But how the activations and gates' values of LSTM are changed for different input data is determined by the LSTM weights which are trained during meta-training and they are fixed through meta-testing. 
The meta version of the three original axioms become as follows.
\\

\noindent \textbf{Meta-Scale-Invariance.} For any $\alpha > 0$, $\mathcal{M}[d](d) = \mathcal{M}[\alpha d](\alpha d)$.
    \\
    
\noindent \textbf{Meta-Richness.} For any finite $X$ and clustering $C$ of $X$, there exists $d \in D(X)$ such that $\mathcal{M}[d](d) = \mathcal{C}$.
    \\
    
\noindent \textbf{Meta-Consistency.} Let $d, d' \in D(X)$ such that $\mathcal{M}[d](d) = \mathcal{C}$ and for all $x, x' \in X$, if $x, x'$ are in the same cluster in $C$ then $d'(x, x') \leq d(x, x')$ while if $x, x'$ are in different clusters in $\mathcal{C}$, then $d'(x,x') \geq d(x,x')$. Then, $\mathcal{M}[d](d') = \mathcal{M}[d](d)$.
\\

    The original consistency axiom demands $\mathcal{A}(d) = \mathcal{A}(d')$, where $d'$ can shrink the distances of points within a cluster and expand the distances between data points in different clusters. It makes sense with respect to the clustering $\mathcal{C} = \mathcal{A}(d)$. In other words, we view $d'$ as a change to $d$ but it could also be viewed as a change from a different distance function $d''$. These two paths ($d'' - d'$ and $d - d'$) can demand $\mathcal{A}(d')$ to have different results because the reference is unclear. By introducing a level of indirection through meta-learning, we can fix the clustering algorithm $\mathcal{A}$ with respect to a reference distance function $d$.
\\

\begin{theorem}
There is a meta clustering algorithm that satisfies Meta-Scale-Invariant and Meta-Richness, Meta-Consistency for $|X| > 2$.
%\TODO{the proof has been changed}
\end{theorem}

\begin{proof}
    We will use the class of single-linkage clusterings parameterized by the threshold.  \textit{Notice how meta scale-invariant axiom and meta richness axiom are just the original axioms but with a level of indirection}. As shown in the Kleinberg's paper, we can use single-linkage clustering with scale-$\alpha$ stopping condition to achieve this (assume there are at least 3 data points and $\alpha < 1$). But single-linkage clustering also directly corresponds to meta clustering with a slight modification by taking two distance functions $d, d'$ (when $d$ = $d'$, it is the original algorithm). The meta step corresponds to the stopping condition that basically finds the maximum pairwise distance $p$ of $d$ , and uses $\alpha p$ ($\alpha$ is a parameter) as the threshold of single-linkage clustering, i.e. $\mathcal{M}[d]$. And the second step uses this threshold to cluster $d'$, i.e. $\mathcal{A}(d)$. The indirection comes to play for the third axiom. It is easy to see that the threshold returned by $\mathcal{M}[d]$ works the same on $d'$.
\end{proof}
